# Supplementary material for: Step by Step to Fairness: Attributing Societal Bias in Task-oriented Dialogue Systems
Source: arXiv:2311.06513 source file (2023-11-14)
Supplement: Supplementary file 1 [file appendix.tex]

\section{Example Appendix}
\label{sec:appendix}

This is an appendix.
